# Supplementary material for: Controlled abstention neural networks for identifying skillful predictions for regression problems
Source: arXiv:2104.08236 ancillary file (2021-04-16)
Supplement: Supplementary file 1 [file Barnes_Barnes_2021_suppRegress.pdf]

# Supporting Information for “Controlled abstention neural networks for identifying skillful predictions for regression problems”

Elizabeth A. Barnes<sup>1</sup> and Randal J. Barnes<sup>2</sup>

<sup>1</sup>Department of Atmospheric Science, Colorado State University, Fort Collins, CO, USA.

<sup>2</sup>Civil, Environmental, and Geo- Engineering, University of Minnesota, Minneapolis, MN, USA.

## Contents of this file

1. Figure S1

---

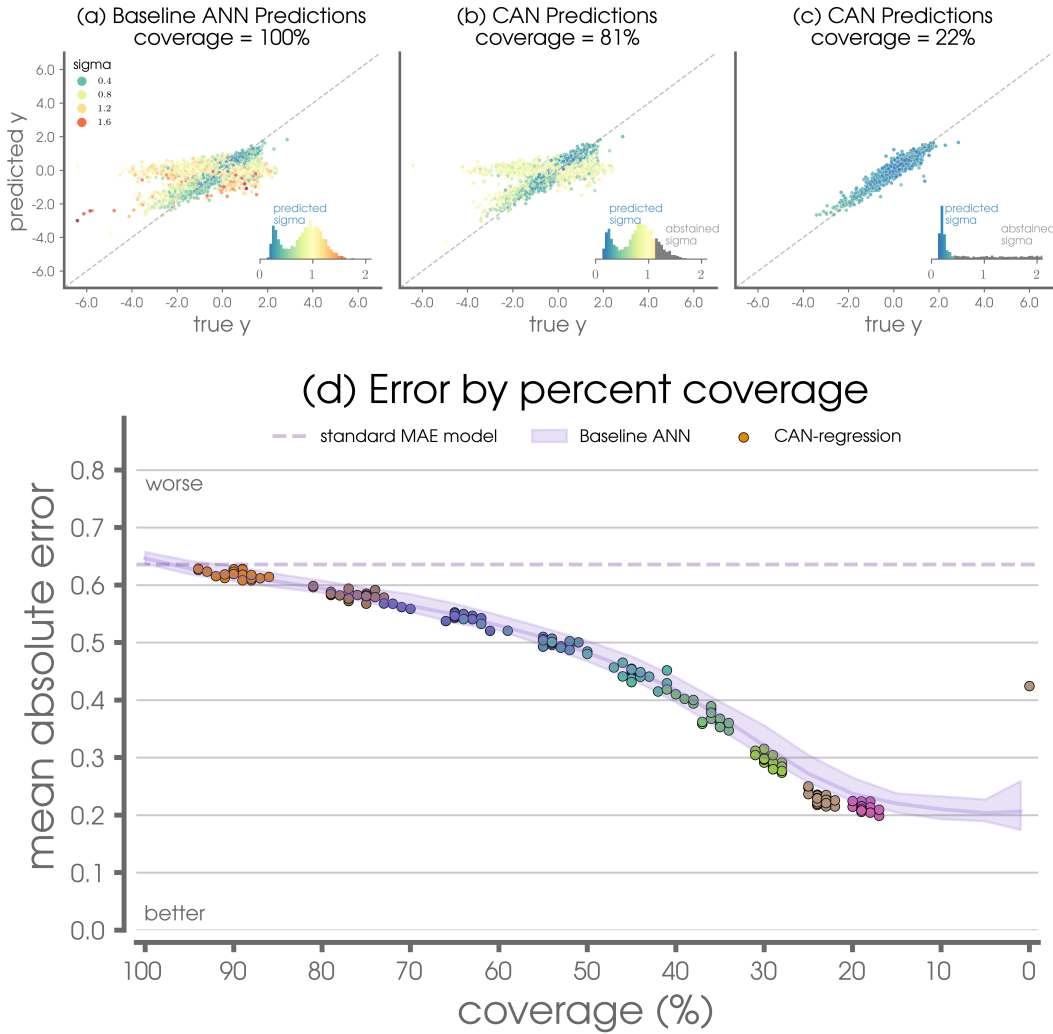

**Figure S1. Forecasts Of Opportunity Experiment w/ Ridge Regression.** (a) Predicted  $y$  versus the true  $y$  for the baseline ANN predictions. The dashed line denotes the one-to-one line, and thus, a perfect prediction. (b,c) As in (a) but for CAN predictions at two different coverage rates. The scatter plots only show covered predictions (i.e. non-abstained). Colors in (a)-(c) denote the predicted  $\sigma$ , and insets in (a)-(c) display histograms of the predicted  $\sigma$  for both covered and abstained predictions. (d) Mean absolute error versus coverage for different neural network loss functions over a range of initialization seeds and abstention setpoints (shown in colors). Purple shading denotes the full range of errors over 20 baseline ANN models with the solid purple line denoting the median.
